# Supplementary material for: Adjacent Leader Decentralized Stochastic Gradient Descent
Source: arXiv:2405.11389 source file (2024-08-19)
Supplement: Supplementary file 1 [file appendix.tex]

% \onecolumn
\hrule height 4pt
\vskip 0.15in
\vskip -\parskip
\begin{center}
{\LARGE\bf Adjacent Leader Decentralized Stochastic Gradient Descent \par} 
\end{center}
\vskip 0.25in
\vskip -\parskip
\hrule height 1pt

\noindent\begin{minipage}{\textwidth}
    \centering
    \includegraphics[width=175mm]{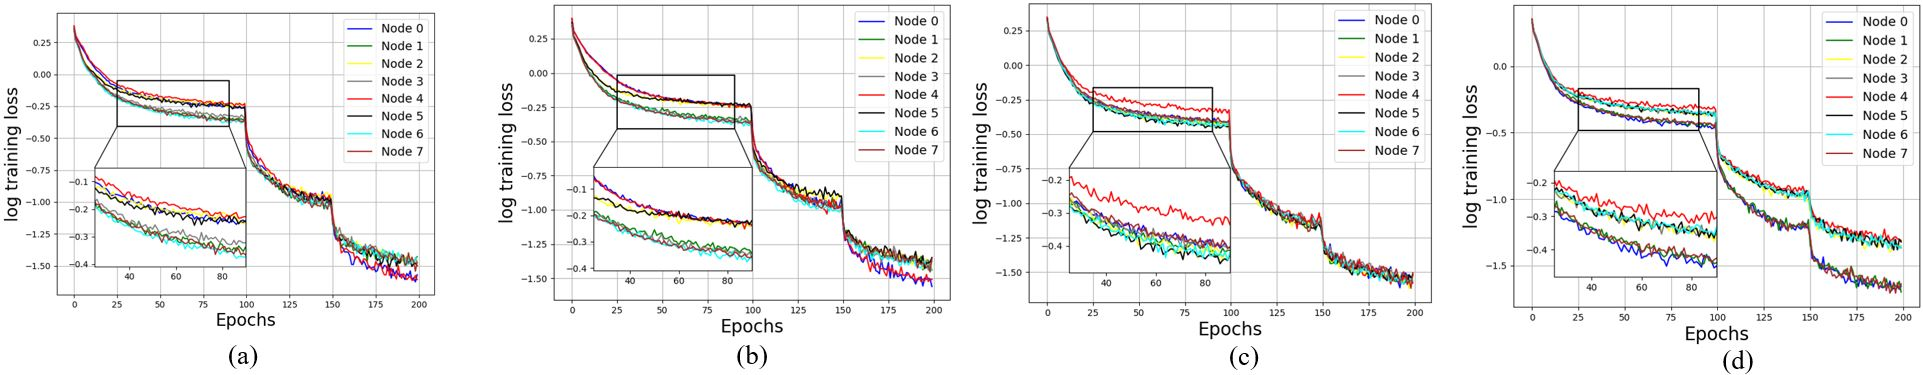}
    \centering
    \captionof{figure}{AL-DSGD without dynamic communication graph. (a): Use D-PSGD as baseline (b):Use MATCHA as baseline.}
    \label{Fig: 9}
\end{minipage}

\section{Dynamic Communication Graphs}\label{Appendix: 1}
We choose pulling coefficients $\lambda_N = 0.1$ and $\lambda_{\tau} = 0.1$. The results can be found in figure~\ref{Fig: 9}. We set model weights coefficients $w_N = 0.1$ and $w_\tau = 0.1$. Without dynamic communication graphs, when applying addictive force according to loss performance, the worker with worse performance and smaller local training loss will affect other nodes. The final test accuracy of the worker with less degree did not improve.

\section{Rotation Subsets}\label{Appendix: 2}
Rotation subsets will assign each worker a new subset in every single iteration. By doing this, we can address the over-fitting problem on worker with worse performance and may achieve faster convergence. We choose pulling coefficients $\lambda_N = 0.1$ and $\lambda_{\tau} = 0.1$. We set model weights coefficients $w_N = 0.1$ and $w_\tau = 0.1$. The results can be found in figure~\ref{Fig: 10}. By applying rotation subsets, we solve the over-fitting problem on worker 0 and worker 4. However, rotation subsets won't accelerate the convergence since the worker 4 still have less communication with other workers. The final test accuracy did not improve on the node with less degree.
\begin{figure}[H]
    \centering
    \includegraphics[width=70mm]{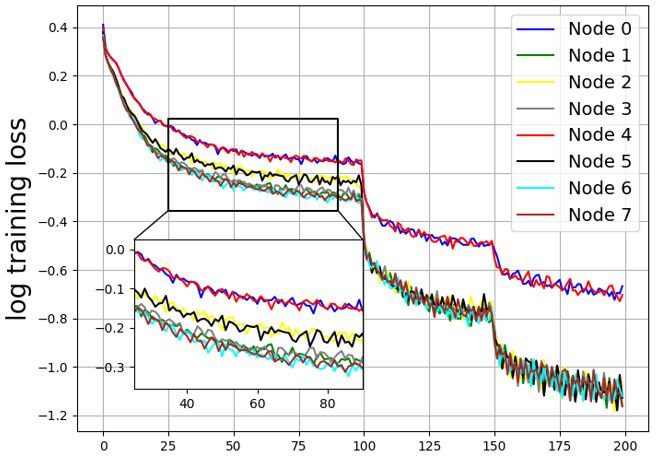}
    \caption{The similarity between dog a and cat b is higher than similarity between b and c. Similarity is calculated using cosine similarity and aussian kernel with L2 distance}
    \label{Fig: 10}
\end{figure}

\section{Proof for Theorem \ref{thm:1}}
In this section, we are going to find a range of $\alpha$, and some averaging hyperparameter $\omega$, such that the spectral norm $\rho=\norm{\mathbb{E}\left[\left(\widetilde{W}^{(k)}-J\right)^\intercal\left(\widetilde{W}^{(k)}-J\right)\right]}$ is smaller than 1.

Recall the formula of mixing matrix $\widetilde{W}^{(k)}$:
\begin{align}\label{eq:W_tilde}
    \widetilde{W}^{(k)}&=(1-\omega_N-\omega_\tau)W^{(k)}+\omega_NA_k^N+\omega_\tau A_k^\tau.
\end{align}
Let $A^{(k)}=\frac{A_k^N+A_k^\tau}{2}$, $\omega=2\omega_N=2\omega_\tau$, we have
\begin{align}\label{eq:W_tilde2}
    \widetilde{W}^{(k)}&=(1-\omega)W^{(k)}+\omega A^{(k)},
\end{align}
where $A$ is still a right stochastic matrix. Therefore:
\begin{align}\label{eq:w-j_1}
    \left(\widetilde{W}^{(k)}-J\right)^\intercal\left(\widetilde{W}^{(k)}-J\right)&=\left(\widetilde{W}^{(k)}^\intercal\widetilde{W}^{(k)}-J\right)-\left(\widetilde{W}^{(k)}^\intercal J-J\right)-\left(J^\intercal\widetilde{W}^{(k)}-J\right)\notag\\
    &=\left(\widetilde{W}^{(k)}^\intercal\widetilde{W}^{(k)}-J\right)-\left(\widetilde{W}^{(k)}-I\right)^\intercal J-J^\intercal\left(\widetilde{W}^{(k)}-I\right).
\end{align}
Since
\begin{align}
    \widetilde{W}^{(k)}-I&=(1-\omega)W^{(k)}+\omega A^{(k)}-I\notag\\
    &=(1-\omega)(I-\alpha L^{(k)})+\omega A^{(k)}-I\notag\\
    &=-\alpha(1-\omega)L^{(k)}+\omega (A^{(k)}-I),
\end{align}
and $L^{k}$ is symmetric and $L^{k}J=0$, we have
\begin{align}
    \left(\widetilde{W}^{(k)}-I\right)^\intercal J &= -\alpha(1-\omega)L^{(k)}J+\omega(A^{(k)}-I)^\intercal J = \omega(A^{(k)}-I)^\intercal J\label{eq:j1}\\
    J^\intercal\left(\widetilde{W}^{(k)}-I\right) &= -\alpha(1-\omega)J^\intercal L^{(k)}+\omega(A^{(k)}-I)^\intercal J = \omega J^\intercal(A^{(k)}-I).\label{eq:j2}
\end{align}
Combine (\ref{eq:w-j_1}), (\ref{eq:j1}) and (\ref{eq:j2}), we have
\begin{align}\label{ieq:W_tilde}
    \norm{\mathbb{E}\left[\left(\widetilde{W}^{(k)}-J\right)^\intercal\left(\widetilde{W}^{(k)}-J\right)\right]}&\leq\norm{\mathbb{E}\left[\widetilde{W}^{(k)}^\intercal\widetilde{W}^{(k)}\right]-J}+2\omega\norm{\mathbb{E}\left[A^{(k)}\right]-I}\norm{J}\notag\\
    &\leq\norm{\widetilde{W}^{(k)}^\intercal\widetilde{W}^{(k)}-J}+2\omega\left(\norm{\mathbb{E}\left[A^{(k)}\right]}+\norm{I}\right)\norm{J}
\end{align}
By the property for spectral norm $\norm{\cdot}\leq\sqrt{\norm{\cdot}_1\norm{\cdot}_1}$, $J=\frac{1}{m}\mathbf{1}\mathbf{1}^\intercal$ and $A^{(k)}$ is left stochastic matrix (after taking expectation $\mathbb{E}\left[A^{(k)}\right]$ is still a left stochastic matrix), we have
\begin{align}\label{ieq:J_A}
    \norm{J}\leq{1},\quad\norm{\mathbb{E}\left[A^{(k)}\right]}\leq\sqrt{m}.
\end{align}
Combine (\ref{ieq:W_tilde}) with (\ref{ieq:J_A}), we have
\begin{align}\label{ieq:W_tilde2}
\norm{\mathbb{E}\left[\left(\widetilde{W}^{(k)}-J\right)^\intercal\left(\widetilde{W}^{(k)}-J\right)\right]}&\leq\norm{\mathbb{E}\left[\widetilde{W}^{(k)}^\intercal\widetilde{W}^{(k)}\right]-J}+2\omega(\sqrt{m}+1).
\end{align}
Then we are going to bound the first part of the RHS of inequality (\ref{ieq:W_tilde2}). Since
\begin{align}\label{ieq:W_tilde_new}
    \norm{\mathbb{E}\left[\widetilde{W}^{(k)}^\intercal\widetilde{W}^{(k)}\right]-J} =& \norm{\mathbb{E}\left[\left[(1-\omega)W^{(k)}+\omega A^{(k)}\right]^\intercal\left[(1-\omega)W^{(k)}+\omega A^{(k)}\right]\right]-J}\notag\\
    \leq&(1-\omega)^2\norm{\mathbb{E}\left[W^{(k)}^\intercal W^{(k)}\right]-J}+\omega(1-\omega)\norm{\mathbb{E}[W^{(k)}^\intercal A^{(k)}]-J}\notag\\
    &+\omega(1-\omega)\norm{\mathbb{E}[A^{(k)}^\intercal W^{(k)}]-J}+\omega^2\norm{A^{(k)}^\intercal A^{(k)}-J}.
\end{align}
We are going to bound each term in iequality (\ref{ieq:W_tilde_new}) one by one.

\textbf{(1) Bound }$\norm{\mathbb{E}\left[W^{(k)}^\intercal W^{(k)}\right]-J}$. 
\begin{align}\label{eq:norm_W_k}
    \norm{\mathbb{E}\left[W^{(k)}^\intercal W^{(k)}\right]-J}=&\norm{\mathbb{E}\left[\left(I-\alpha L^{(k)}\right)^\intercal \left(I-\alpha L^{(k)}\right)\right]-J}\notag\\
    =&\norm{I-2\alpha\mathbb{E}\left[L^{(k)}\right]+\alpha^2\mathbb{E}\left[L^{(k)}^\intercal L^{(k)}\right]-J}.
\end{align}
Recall there are two communication graph and $L^{(k)}$ is periodically switched between them:
$$ L^{(k)}=\left\{
\begin{aligned}
\sum_{j=1}^mB^{(k)}_{(1),j}L_{(1),j} \quad& \text{if k is odd,}&\\
\sum_{j=1}^mB^{(k)}_{(2),j}L_{(2),j} \quad& \text{if k is even,}&
\end{aligned}
\right.
$$
We are going to analysis them separately.
\begin{itemize}
    \item If $k$ is odd. Then we have
    \begin{align*} \mathbb{E}\left[L^{(k)}\right]&=\sum_{j=1}^mp_{(1),j}L_{(1),j}\\
        \mathbb{E}\left[L^{(k)}^\intercal L^{(k)}\right]&=\sum_{j=1}^mp_{(1),j}^2L_{(1),j}^2+\sum_{j=1}^M\sum_{t=1,t\neq j}^Mp_{(1),j}p_{(1),t}L_{(1),j}^\intercal L_{(1),t}+\sum_{j=1}^Mp_{(1),j}(1-p_{(1),j})L_{(1),j}\\
        &=\left(\sum_{j=1}^mp_{(1),j}L_{(1),j}\right)^2+2\sum_{j=1}^Mp_{(1),j}(1-p_{(1),j})L_{(1),j}
    \end{align*}
    Therefore, we have
    \begin{align}
    \norm{\mathbb{E}\left[W^{(k)}^\intercal W^{(k)}\right]-J}\leq&\norm{\left(I-\alpha\sum_{j=1}^mp_{(1),j}L_{(1),j}\right)^2}+2\alpha^2\norm{2\sum_{j=1}^Mp_{(1),j}(1-p_{(1),j})L_{(1),j}}\notag\\
        =&\max\{(1-\alpha\lambda_{(1),2})^2,(1-\alpha\lambda_{(1),m})^2\}+2\alpha^2\zeta_{(1)},
    \end{align}
    where $\lambda_{(1),i}$ denote the $i$-th smallest eigenvalue of matrix $\sum_{j=1}^mp_{(1),j}L_{(1),j} $ and $\zeta_{(1)}>0$ denote the spectral norm of matrix $\sum_{j=1}^mp_{(1),j}(1-p_{(1),j})L_{(1),j}$.
    
    \item If $k$ is even.
    Similarly, we could conclude:
    \begin{align}
        \norm{\mathbb{E}\left[W^{(k)}^\intercal W^{(k)}\right]-J}\leq\max\{(1-\alpha\lambda_{(2),2})^2,(1-\alpha\lambda_{(2),m})^2\}+2\alpha^2\zeta_{(2)},
    \end{align}
    where $\lambda_{(2),i}$ denote the $i$-th smallest eigenvalue of matrix $\sum_{j=1}^mp_{(2),j}L_{(2),j} $ and $\zeta_{(2)}>0$ denote the spectral norm of matrix $\sum_{j=1}^mp_{(2),j}(1-p_{(2),j})L_{(2),j}$.
\end{itemize}
In all, we could conclude
\begin{align}       &\norm{\mathbb{E}\left[W^{(k)}^\intercal W^{(k)}\right]-J}\notag\\
        \leq&\max\{(1-\alpha\lambda_{(1),2})^2,(1-\alpha\lambda_{(1),m})^2,(1-\alpha\lambda_{(2),2})^2,(1-\alpha\lambda_{(2),m})^2\}+2\alpha^2\max\{\zeta_{(1)},\zeta_{(2)}\}.
\end{align}

Assume $\lambda$ represents the eigenvalue such that $|1-\alpha\lambda|=\max\{|1-\alpha\lambda_{(1),2}|,|1-\alpha\lambda_{(1),m}|,|1-\alpha\lambda_{(2),2}|,|1-\alpha\lambda_{(2),m}|\}$, and $\zeta=\max\{\zeta_{(1)},\zeta_{(2)}\}$, we could have

\begin{align}       \norm{\mathbb{E}\left[W^{(k)}^\intercal W^{(k)}\right]-J}\leq|1-\alpha\lambda|^2+2\alpha^2\zeta.
\end{align}

\textbf{(2) Bound} $\norm{\mathbb{E}[W^{(k)}^\intercal A^{(k)}]-J}$ and $\norm{\mathbb{E}[A^{(k)}^\intercal W^{(k)}]-J}$.
\begin{align}
    \norm{\mathbb{E}[W^{(k)}^\intercal A^{(k)}]-J}=&\norm{\mathbb{E}\left[W^{(k)}^\intercal A^{(k)}-J\right]}\notag\\
    =&\norm{\mathbb{E}\left[W^{(k)}^\intercal (A^{(k)}-J)\right]}\notag\\
    \leq&(\sqrt{m}+1)\norm{I-\alpha\mathbb{E}[L^{(k)}]}
\end{align}
Similarly to the proof in \textbf{(1)}, we could conclude:
\begin{align}
    \norm{\mathbb{E}[W^{(k)}^\intercal A^{(k)}]-J}\leq(\sqrt{m}+1)|1-\alpha\lambda|,
\end{align}
where $\lambda$ represents the eigenvalue such that $|1-\alpha\lambda|=\max\{|1-\alpha\lambda_{(1),2}|,|1-\alpha\lambda_{(1),m}|,|1-\alpha\lambda_{(2),2}|,|1-\alpha\lambda_{(2),m}|\}$. Similarly, we could bound $\norm{\mathbb{E}[A^{(k)}^\intercal W^{(k)}]-J}$.

\textbf{(3) Bound} $\norm{A^{(k)}^\intercal A^{(k)}-J}$.
Denote $B^{(k)}=A^{(k)}^\intercal A^{(k)}$. Denote $a_{ij}^{(k)}$ and $b_{ij}^{(k)}$ be the elemnts of matrix $A^{(k)}$ and $B^{(k)}$ respectively. Therefore:
\begin{align*}
b_{ij}^{(k)}=\sum_{l=1}^ma_{li}^{(k)}a_{lj}^{(k)}.
\end{align*}
Therefore:
\begin{align*}
    \norm{B^{(k)}}_1=\max_j\sum_{i=1}^m|b_{ij}^{(k)}|=\max_j\sum_{i=1}^m\sum_{l=1}^ma_{li}^{(k)}a_{lj}^{(k)}=\max_j\sum_{l=1}^ma_{lj}^{(k)}\sum_{i=1}^ma_{li}^{(k)}=\max_jm\sum_{l=1}^ma_{lj}^{(k)}\leq m
\end{align*}
Similarly we could conclude $\norm{B^{(k)}}_\infty\leq m$. Therefore, we have
\begin{align*}
    \norm{A^{(k)}^\intercal A^{(k)}-J}\leq\norm{B^{k}}+1\leq m+1.
\end{align*}

Combine \textbf{(1-3)} and (\ref{ieq:W_tilde2}), we have
\begin{align}\label{ieq:W_tilde_new}
    &\norm{\mathbb{E}\left[\left(\widetilde{W}^{(k)}-J\right)^\intercal\left(\widetilde{W}^{(k)}-J\right)\right]}\notag\\
    \leq&(1-\omega)^2|1-\alpha\lambda|^2+2\alpha^2\zeta+2w(1-\omega)(\sqrt{m}+1)|1-\alpha\lambda|+\omega^2(m+1)+2\omega(\sqrt{m}+1).
\end{align}

By the analysis in Appendix B of \cite{wang2019matcha}, we know $\lambda>0$. We assume $\alpha<\frac{1}{\lambda}$ and rewrite the inequality as
\begin{align}\label{ieq:W_tilde_new}
    &\norm{\mathbb{E}\left[\left(\widetilde{W}^{(k)}-J\right)^\intercal\left(\widetilde{W}^{(k)}-J\right)\right]}\notag\\
    \leq&(1-\omega)^2(1-\alpha\lambda)^2+2\alpha^2\zeta+2w(1-\omega)(\sqrt{m}+1)(1-\alpha\lambda)+\omega^2(m+1)+2\omega(\sqrt{m}+1)\notag\\
    =&\left[(1-\omega)(1-\alpha)+\omega(\sqrt{m}+1)\right]^2+2\alpha^2\zeta+2\omega(\sqrt{m}+1)-2\omega^2\sqrt{m}\notag\\
    \leq&\left[(1-\omega)(1-\alpha)+\omega(\sqrt{m}+1)\right]^2+2\alpha^2\zeta+2\omega(\sqrt{m}+1)
\end{align}

Let $\omega=\frac{1-\alpha\lambda}{k(\sqrt{m}+1)}$, where $k>1$. We know that under this definition, $\omega$ is between $0$ and $1$. Then the bound could be rewrite as:
\begin{align}\label{ieq:W_tilde_new}
    &\norm{\mathbb{E}\left[\left(\widetilde{W}^{(k)}-J\right)^\intercal\left(\widetilde{W}^{(k)}-J\right)\right]}\notag\\
    \leq&\left[\frac{k+1}{k}(1-\alpha\lambda)-\frac{1-\alpha\lambda}{k(\sqrt{m}+1)}\right]^2+\frac{2(1-\alpha\lambda)}{k}+2\alpha^2\zeta\notag\\
    \leq&\frac{(k+1)^2}{k^2}(1-\alpha\lambda)^2+\frac{2(1-\alpha\lambda)}{k}+2\alpha^2\zeta.
\end{align}
Define $h_\lambda(\alpha)=\frac{(k+1)^2}{k^2}(1-\alpha\lambda)^2+\frac{2(1-\alpha\lambda)}{k}+2\alpha^2\zeta$, then we have
\begin{align*}
    h'_{\lambda}(\alpha)&=-\frac{2(k+1)^2}{k^2}\lambda(1-\alpha\lambda)-\frac{2\lambda}{k}+4\alpha\zeta,\\
    h''_{\lambda}(\alpha)&=\frac{2(k+1)^2}{k^2}\lambda^2+4\zeta.
\end{align*}
Since $h''_\lambda(\alpha)>0$, $h_\lambda(\alpha)$ is convex quadratic fucntion. Let $h'_\lambda(\alpha)=0$, we could get the minimun point is:
$$\alpha^*=\frac{[(k+1)^2+k]\lambda}{(k+1)^2\lambda^2+2k^2\zeta}.$$
We take $\widetilde{\alpha}=\frac{(k+1)^2\lambda}{(k+1)^2\lambda+2k^2\zeta},$ it is easy to know $\widetilde{\alpha}<\alpha^*$.
\begin{align*}
    h_\lambda(\widetilde{\alpha})=\frac{(k+1)^2}{k^2}(1-\widetilde{\alpha}\lambda)^2+\frac{2}{k}(1-\widetilde{\alpha}\lambda)+2\alpha^2\zeta=\frac{4k\zeta+2(k+1)^2\zeta}{(k+1)^2\lambda^2+2k^2\zeta}.
\end{align*}

Now, when $k>\max\{1, \frac{2\zeta}{\lambda^2}-1, \frac{\lambda(\lambda-1)}{2\zeta}\}$, we have $\widetilde{\alpha}<\frac{1}{\lambda}$ and $h_\lambda(\widetilde{\alpha})<1$. Take a rational k, by the convex property of $h_{\lambda}(\alpha)$, we know when $\alpha\in\left(\alpha_{min}, \alpha_{max}\right)$, where:
\begin{align*}
    \alpha_{min} = \frac{(k+1)^2\lambda}{(k+1)^2\lambda+2k^2\zeta},\quad
    \alpha_{max} = \min\{\frac{1}{\lambda}, \frac{[(k+1)^2+k]\lambda}{(k+1)^2\lambda+2k^2\zeta}\}.
\end{align*}
There exists an averaging parameter
$\omega(\alpha)=\frac{1-\alpha\lambda}{k(\sqrt{m}+1)}$, such that
$$\norm{\mathbb{E}\left[\left(\widetilde{W}^{(k)}-J\right)^\intercal\left(\widetilde{W}^{(k)}-J\right)\right]}\leq h_\lambda(\alpha)<1$$.

\section{Proof for Theorem \ref{thm:2}}
\subsection{Lemmas}
Befor moving into the detailed proof, we first introduce a lemma.
\begin{lemma}\label{lma:1}
    Let $\{\widetilde{w}^{(k)}\}_{k=1}^{infty}$ be i.i.d right stochastic matrices sequence with property $$\rho=\norm{\mathbb{E}\left[\left(\widetilde{W}^{(k)}-J\right)^\intercal\left(\widetilde{W}^{(k)}-J\right)\right]}<1,$$
    Then we could claim
    \begin{align*}
        \mathbb{E}\left[\norm{B\prod_{k=1}^n(\widetilde{W}^{(k)}-J)}_F^2\right]\leq\rho^n\norm{B}_F^2.
    \end{align*}
\end{lemma}
\begin{proof}[Proof for Lemma \ref{lma:1}.]
Define $A_{q,n}=\prod_{k=q}^n(\widetilde{W}^{(k)}-J)$, $b_i^\interval$ denote the $i$-th row vector of $B$. Thus, we have
$$A_{1,n}=A_{1,n-1}\left(W^{(n)}-J\right).$$
Thus, we have
\begin{align*}
    \mathbb{E}_{\widetilde{W}^{(n)}}\left[\norm{BA_{1,n}}_F^2\right]\leq&\sum_{i=1}^d\mathbb{E}_{\widetilde{W}^{(n)}}\left[\norm{b_i^\intercal A_{1,n}}^2\right]\notag\\
    \leq&\sum_{i=1}^d\mathbb{E}_{\widetilde{W}^{(n)}}\left[b_i^\intercal A_{1,n-1}\left(\widetilde{W}^{(n)}-J\right)^\intercal\left(\widetilde{W}^{(n)}-J\right)A_{1,n-1}^\intercal b_i\right]\notag\\
    =&\sum_{i=1}^db_i^\intercal A_{1,n-1}\mathbb{E}_{\widetilde{W}^{(n)}}\left[\left(\widetilde{W}^{(n)}-J\right)^\intercal\left(\widetilde{W}^{(n)}-J\right)\right]A_{1,n-1}^\intercal b_i.
\end{align*}
Let$C=\mathbb{E}_{\widetilde{W}^{(n)}}\left[\left(\widetilde{W}^{(n)}-J\right)^\intercal\left(\widetilde{W}^{(n)}-J\right)\right]$, $v_i=A_{1,n-1}^\intercal b_i$, therefore we have:
\begin{align*}
    \mathbb{E}_{\widetilde{W}^{(n)}}\left[\norm{BA_{1,n}}_F^2\right]\leq\sum_{i=1}^d\mathbb{E}_{\widetilde{W}^{(n)}}\left[\norm{b_i^\intercal A_{1,n}}^2\right]=&\sum_{i=1}^dv_i^\intercal C v_i
    \leq \sigma)\max(C)\sum_{i=1}^dv_i^\intercal v_i=\rho\norm{BA_{1,n-1}}_F^2
\end{align*}
Therefore, we have
\begin{align*}
        \mathbb{E}_{\widetilde{W}^{(1)},...,\widetilde{W}^{(n)}}\left[\norm{B\prod_{k=1}^n(\widetilde{W}^{(k)}-J)}_F^2\right]\leq\rho^n\norm{B}_F^2.
    \end{align*}
\end{proof}

\subsection{Detailed proof of Theorem \ref{thm:2}}
Recall the update rule for AL-DSGD algorithm:
\begin{align}
    X_{k+1}=\widetilde{W}^{k}X_{k}-\eta\left[G^{(k)}+\lambda_N(X_{k+\frac{1}{2}}-X_k^N)+\lambda_\tau(X_{k+\frac{1}{2}}-X_k^\tau)\right],
\end{align}
where 
\begin{align*}
    X_k &= [x_{1,k},...,x_{m,k}],\\
    G^{(k)} &= [g_1(x_{1,k}),...,g_m(x_{m,k})],\\
    \nabla F^{(k)}&=[\nabla F_1(x_{1,k}),...,\nabla F_m(x_{m,k})]
\end{align*}
Let $\lambda=2\lambda_N=2\lambda_\tau$, and $C_k = \frac{1}{2}(X_k^N+X_k^\tau)$. Then we have
\begin{align}
    X_{k+1}=\widetilde{W}^{k}X_{k}-\eta\left[G^{(k)}+\lambda(X_{k+\frac{1}{2}}-C_k)\right]
\end{align}
After taking the average we have
\begin{align}
    \overline{x}_{k+1}=\overline{x}_k-\eta\left[\frac{G^{(k)}\mathbf{1}}{m}+\lambda(\overline{x}_{k+\frac{1}{2}}-\overline{c}_k)\right]=\overline{x}_k-\eta\left[\frac{G^{(k)}\mathbf{1}}{m}+\lambda\Delta_k\right].
\end{align}
Denote $\Delta_k = \overline{x}_{k+\frac{1}{2}}-\overline{c}_k$. 
from Assumption \ref{asm:1} (5), we could conclude $\norm{\Delta_k}^2\leq\delta^2$.

Then we have
\begin{align}
    F(\overline{x}_{k+1})-F(\overline{x}_{k})\leq& \langle\nabla F(\overline{x}_k), \overline{x}_{k+1}-\overline{x}_k\rangle+\frac{L}{2}\norm{\overline{x}_{k+1}-\overline{x}_k}\notag\\
    \leq&-\eta\langle\nabla F(\overline{x}_k), \frac{G^{(k)}\mathbf{1}}{m}+\lambda\Delta_k\rangle+\frac{\eta^2L}{2}\norm{\frac{G^{(k)}\mathbf{1}}{m}+\lambda\Delta_k}\notag\\
    \leq&-\eta\langle\nabla F(\overline{x}_k), \frac{G^{(k)}\mathbf{1}}{m}\rangle+\frac{\eta^2L}{2}\norm{\frac{G^{(k)}\mathbf{1}}{m}}\notag\\
    &-\lambda\eta\langle\nabla F(\overline{x}_k),\Delta_k\rangle+\frac{\lambda^2\eta^2L}{2}\norm{\Delta_k}^2+\lambda\eta^2L\langle\frac{G^{(k)}\mathbf{1}}{m},\Delta_k\rangle\notag\\
    \leq&-\eta\langle\nabla F(\overline{x}_k), \frac{G^{(k)}\mathbf{1}}{m}\rangle+\frac{\eta^2L}{2}\norm{\frac{G^{(k)}\mathbf{1}}{m}}+\lambda\eta\beta\delta+\lambda\eta^2L\beta \delta+\frac{\lambda^2\eta^2L\delta^2}{2}
\end{align}

Inspired by the proof in Appendix C.3 of \cite{wang2019matcha}, we have:
\begin{align}
    \mathbb{E}\left[F(\overline{x}_{k+1})-F(\overline{x}_{k})\right]\leq&-\frac{\eta}{2}\mathbb{E}\left[\norm{\nabla F(\overline{x}_k)}^2\right]-\frac{\eta}{2}(1-\eta L)\mathbb{E}\left[\norm{\frac{\nabla F^{(k)}\mathbf{1}}{m}}^2\right]\\
    &+\frac{\eta L^2}{2m}\mathbb{E}\left[\norm{X_k(I-J)}_F^2\right]+\frac{\eta^2L\sigma^2}{2m}+\lambda\eta\beta\delta+\lambda\eta^2L\beta \delta+\frac{\lambda^2\eta^2L\delta^2}{2}
\end{align}

Denote $M=\frac{\eta^2L\sigma^2}{2m}+\lambda\eta\beta\delta+\lambda\eta^2L\beta \delta+\frac{\lambda^2\eta^2L\delta^2}{2}$, the bound could be simplified as
\begin{align}
    \mathbb{E}\left[F(\overline{x}_{k+1})-F(\overline{x}_{k})\right]\leq-\frac{\eta}{2}\mathbb{E}\left[\norm{\nabla F(\overline{x}_k)}^2\right]-\frac{\eta}{2}(1-\eta L)\mathbb{E}\left[\norm{\frac{\nabla F^{(k)}\mathbf{1}}{m}}^2\right]+\frac{\eta L^2}{2m}\mathbb{E}\left[\norm{X_k(I-J)}_F^2\right]+M.
\end{align}
Summing over all iterations and then take the average, we have
\begin{align}
    \frac{\mathbb{E}\left[F(\overline{x}_{K})-F(\overline{x}_{1})\right]}{K}
    \leq& -\frac{\eta}{2}\frac{1}{K}\sum_{k=1}^k\mathbb{E}\left[\norm{\nabla F(\overline{x}_k)}^2\right]-\frac{\eta}{2}(1-\eta L)\frac{1}{K}\sum_{k=1}^k\mathbb{E}\left[\norm{\frac{\nabla F^{(k)}\mathbf{1}}{m}}^2\right]\notag\\
    &+\frac{\eta L^2}{2mK}\sum_{k=1}^k\mathbb{E}\left[\norm{X_k(I-J)}_F^2\right]+M.
\end{align}
By rearranging the inequality, we have
\begin{align}\label{ieq:sumF1}
    \frac{1}{K}\sum_{k=1}^k\mathbb{E}\left[\norm{\nabla F(\overline{x}_k)}^2\right]
    \leq&\frac{2(F(\overline{x}_{1})-F^*)}{\eta K}-(1-\eta L)\frac{1}{K}\sum_{k=1}^k\mathbb{E}\left[\norm{\frac{\nabla F^{(k)}\mathbf{1}}{m}}^2\right]\notag\\
    &+\frac{L^2}{mK}\sum_{k=1}^k\mathbb{E}\left[\norm{X_k(I-J)}_F^2\right]+\frac{2M}{\eta}\notag\\
    \leq&\frac{2(F(\overline{x}_{1})-F^*)}{\eta K}+\frac{L^2}{mK}\sum_{k=1}^k\mathbb{E}\left[\norm{X_k(I-J)}_F^2\right]+\frac{2M}{\eta}.
\end{align}
Then we are goint to bound $\mathbb{E}\left[\norm{X_k(I-J)}_F^2\right]$. By the property of matrix $J$, we have
\begin{align}
    X_k(I-J)=&(X_{k-1}-\eta(G^{(k-1)}+\lambda\Delta_{k-1})\widetilde{W}^{(k-1)}(I-J)\notag\\
    =&X_{k-1}(\widetilde{W}^{(k-1)}-J)-\eta(\G^{(k-1)}+\lambda\Delta^{(k-1)})(\widetilde{W}^{(k-1)}-J)
    =&...\notag\\
    =&X_{1}\prod_{q=1}^{k-1}(\widetilde{W}^{(q)}-J)-\eta \sum_{q=1}^{k-1}(G^{(k-1)}+\lambda\Delta^{(k)})\prod_{l=q}^{k-1}(\widetilde{W}^{(l)}-J)
\end{align}
Without loss of generalizty, assume $X_{1}=0$. Therefore, by Assumption (\ref{asm:1}) and Lemma \ref{lma:1} we have
\begin{align}
    \norm{X_k(I-J)}_F^2=&\eta^2\norm{\sum_{q=1}^{k-1}(G^{(k-1)}+\lambda\Delta^{(k)})\prod_{l=q}^{k-1}(\widetilde{W}^{(l)}-J)}_F^2\notag\\
    \leq&2\eta^2\norm{\sum_{q=1}^{k-1}G^{(k-1)}\prod_{l=q}^{k-1}(\widetilde{W}^{(l)}-J)}_F^2+2\eta^2\lambda^2\norm{\sum_{q=1}^{k-1}\Delta^{(k)}\prod_{l=q}^{k-1}(\widetilde{W}^{(l)}-J)}_F^2\notag\\
    \leq&2\eta^2\norm{\sum_{q=1}^{k-1}G^{(k-1)}\prod_{l=q}^{k-1}(\widetilde{W}^{(l)}-J)}_F^2+2\eta^2\lambda^2\delta^2\sum_{q=1}^k\rho^q\notag\\
    \leq&2\eta^2\norm{\sum_{q=1}^{k-1}G^{(k-1)}\prod_{l=q}^{k-1}(\widetilde{W}^{(l)}-J)}_F^2+\frac{2\eta^2\lambda^2\delta^2\rho}{1-\rho}\notag\\
    \leq&2\eta^2\norm{\sum_{q=1}^{k-1}\left(G^{(k-1)}-\nabla F^{(q)}\right)\prod_{l=q}^{k-1}(\widetilde{W}^{(l)}-J)}_F^2+2\eta^2\norm{\sum_{q=1}^{k-1}\nabla F^{(q)}\prod_{l=q}^{k-1}(\widetilde{W}^{(l)}-J)}_F^2+\frac{2\eta^2\lambda^2\delta^2\rho}{1-\rho}.
\end{align}
Taking expectation, we have:
\begin{align}
    \mathbb{E}\left[\norm{X_k(I-J)}_F^2\right]\leq 2\eta^2\mathbb{E}\left[\norm{\sum_{q=1}^{k-1}\nabla F^{(q)}\prod_{l=q}^{k-1}(\widetilde{W}^{(l)}-J)}_F^2\right] +\frac{2m\eta^2\sigma^2\rho}{1-\rho}+\frac{2\eta^2\lambda^2\delta^2\rho}{1-\rho}
\end{align}
For notation simplicity, let $B_{q,p}=\prod_{l=q}^p(\widetilde{W}^{(l)}-J)$, then we have
\begin{align}
    &\mathbb{E}\left[\norm{\sum_{q=1}^{k-1}\nabla F^{(q)}\prod_{l=q}^{k-1}(\widetilde{W}^{(l)}-J)}_F^2\right]\notag\\
    =&\sum_{q=1}^{k-1}\mathbb{E}\left[\norm{\nabla F^{(q)}B_{q,k-1}}_F^2\right]+\sum_{q=1}^{k-1}\sum_{p=1,p\neq q}^{k-1}\mathbb{E}\left[Tr\{B_{q,k-1}^\intercal\nabla F^{(q)}^\intercal\nabla F^{(p)}B_{p,k-1}\}\right]\notag\\
    \leq& \sum_{q=1}^{k-1}\mathbb{E}\left[\norm{\nabla F^{(q)}B_{q,k-1}}_F^2\right]+\sum_{q=1}^{k-1}\sum_{p=1,p\neq q}^{k-1}\mathbb{E}\left[\norm{\nabla F^{(q)}B_{q,k-1}}_F^2\norm{\nabla F^{(p)}B_{p,k-1}}_F^2\right]\notag\\
    \leq&\sum_{q=1}^{k-1}\mathbb{E}\left[\norm{\nabla F^{(q)}B_{q,k-1}}_F^2\right]+\sum_{q=1}^{k-1}\sum_{p=1,p\neq q}^{k-1}\mathbb{E}\left[\frac{1}{2\epsilon}\norm{\nabla F^{(q)}B_{q,k-1}}_F^2+\frac{\epsilon}{2}\norm{\nabla F^{(p)}B_{p,k-1}}_F^2\right]\notag\\
    \leq&\sum_{q=1}^{k-1}\mathbb{E}\left[\norm{\nabla F^{(q)}B_{q,k-1}}_F^2\right]+\sum_{q=1}^{k-1}\sum_{p=1,p\neq q}^{k-1}\mathbb{E}\left[\frac{\rho^{k-q}}{2\epsilon}\norm{\nabla F^{(q)}}_F^2+\frac{\rho^{k-p}\epsilon}{2}\norm{\nabla F^{(p)}}_F^2\right].
\end{align}
Taking $\epsilon=\rho^{\frac{p-q}{2}}$, we have
\begin{align*}
    &\mathbb{E}\left[\norm{\sum_{q=1}^{k-1}\nabla F^{(q)}\prod_{l=q}^{k-1}(\widetilde{W}^{(l)}-J)}_F^2\right]\notag\\
    \leq&\sum_{q=1}^{k-1}\mathbb{E}\left[\norm{\nabla F^{(q)}B_{q,k-1}}_F^2\right]+\frac{1}{2}\sum_{q=1}^{k-1}\sum_{p=1,p\neq q}^{k-1}\sqrt{\rho}^{2k-p-q}\mathbb{E}\left[\norm{\nabla F^{(q)}}_F^2+\norm{\nabla F^{(p)}}_F^2\right]\notag\\
    =&\sum_{q=1}^{k-1}\mathbb{E}\left[\norm{\nabla F^{(q)}B_{q,k-1}}_F^2\right]+\sum_{q=1}^{k-1}\sqrt{\rho}^{k-q}\mathbb{E}\left[\norm{\nabla F^{(q)}}_F^2\right]\sum_{p=1,p\neq q}^{k-1}\sqrt{\rho}^{k-p}\notag\\
    =&\sum_{q=1}^{k-1}\mathbb{E}\left[\norm{\nabla F^{(q)}B_{q,k-1}}_F^2\right]+\sum_{q=1}^{k-1}\sqrt{\rho}^{k-q}\mathbb{E}\left[\norm{\nabla F^{(q)}}_F^2\right]\left(\sum_{p=1}^{k-1}\sqrt{\rho}^{k-p}-\sqrt{\rho}^{k-q}\right)\notag\\
    \leq&\frac{\sqrt{\rho}}{1-\sqrt{\rho}}\sum_{q=1}^{k-1}\sqrt{\rho}^{k-q}\mathbb{E}\left[\norm{\nabla F^{(q)}}_F^2\right].
\end{align*}
Therefore,
\begin{align}
    \mathbb{E}\left[\norm{X_k(I-J)}_F^2\right]\leq\frac{2\eta^2\sqrt{\rho}}{1-\sqrt{\rho}}\sum_{q=1}^{k-1}\sqrt{\rho}^{k-q}\mathbb{E}\left[\norm{\nabla F^{(q)}}_F^2\right] +\frac{2\eta^2\rho(m\sigma^2+\lambda^2\delta^2)}{1-\rho}.
\end{align}
Therefore
\begin{align}
    \frac{1}{mK}\sum_{k=1}^K\mathbb{E}\left[\norm{X_k(I-J)}_F^2\right]\leq&\frac{2\eta^2\sqrt{\rho}}{mK(1-\sqrt{\rho})}\sum_{k=1}^K\sum_{q=1}^{k-1}\sqrt{\rho}^{k-q}\mathbb{E}\left[\norm{\nabla F^{(q)}}_F^2\right] +\frac{2\eta^2\rho(m\sigma^2+\lambda^2\delta^2)}{m(1-\rho)}\notag\\
    \leq&\frac{2\eta^2\sqrt{\rho}}{mK(1-\sqrt{\rho})}\sum_{k=1}^K\frac{\sqrt{\rho}}{1-\sqrt{\rho}}\mathbb{E}\left[\norm{\nabla F^{(q)}}_F^2\right] +\frac{2\eta^2\rho(m\sigma^2+\lambda^2\delta^2)}{m(1-\rho)}\notag\\
    =&\frac{2\eta^2\rho}{mK(1-\sqrt{\rho})^2}\sum_{k=1}^K\mathbb{E}\left[\norm{\nabla F^{(q)}}_F^2\right] +\frac{2\eta^2\rho(m\sigma^2+\lambda^2\delta^2)}{m(1-\rho)}
\end{align}
Note that
\begin{align}
    \norm{\nabla F^{(q)}}_F^2=&\sum_{i=1}^m\norm{\nabla F_i(x_{i,k})}^2\notag\\
    =&\sum_{i=1}^m\norm{\nabla F_i(x_{i,k})-\nabla F(x_{i,k})+\nabla F(x_{i,k})-\nabla F(\overline{x}_k)+\nabla F(\overline{x}_k)}^2\notag\\
    \leq&3\sum_{i=1}^m\left[\norm{\nabla F_i(x_{i,k})-\nabla F(x_{i,k})}^2+\norm{\nabla F(x_{i,k})-\nabla F(\overline{x}_k)}^2+\norm{\nabla F(\overline{x}_k)}^2\right]\notag\\
    \leq&3m\zeta^2+3L^2\norm{X_k(I-J)}_F^2+3m\norm{\nabla F(\overline{x}_k)}^2.
\end{align}
Therefore, we have
\begin{align}
    \frac{1}{mK}\sum_{k=1}^K\mathbb{E}\left[\norm{X_k(I-J)}_F^2\right]\leq&\frac{2\eta^2\rho(m\sigma^2+\lambda^2\delta^2)}{m(1-\rho)}+\frac{6\eta^2\zeta^2\rho}{(1-\sqrt{\rho})^2}+\frac{6\eta^2\zeta^2\rho}{(1-\sqrt{\rho})^2}\frac{1}{mK}\mathbb{E}\left[\norm{X_k(I-J)}_F^2\right]\notag\\
    &+\frac{6\eta^2\rho}{(1-\sqrt{\rho})^2}\frac{1}{K}\sum_{i=1}^K\mathbb{E}\left[\norm{\nabla F(\overline{x}_k)}^2\right].
\end{align}
Define $D=\frac{6\eta^2L^2\rho}{(1-\sqrt{\rho})^2}$, by rearranging we have
\begin{align}\label{ieq:XIJ}
    \frac{1}{mK}\sum_{k=1}^K\mathbb{E}\left[\norm{X_k(I-J)}_F^2\right]\leq\frac{1}{1-2D}\left[\frac{2\eta^2\rho(m\sigma^2+\lambda^2\delta^2)}{m(1-\rho)}+\frac{6\eta^2\zeta^2\rho}{(1-\sqrt{\rho})^2}+\frac{6\eta^2\rho}{(1-\sqrt{\rho})^2}\frac{1}{K}\sum_{i=1}^K\mathbb{E}\left[\norm{\nabla F(\overline{x}_k)}^2\right]\right]
\end{align}
Plugging (\ref{ieq:XIJ}) back to (\ref{ieq:sumF1}), we have
\begin{align}
\frac{1}{K} \sum_{i=1}^K\mathbb{E}\left[\norm{\nabla F(\overline{x}_k)}^2\right]\leq &\frac{2(F(\overline{x}_{1})-F^*)}{\eta K}+\frac{2M}{\eta}+\frac{1}{1-D}\frac{2\eta^2L^2\rho(m\sigma^2+\lambda^2\delta^2)}{m(1-\rho)}+\frac{D\zeta^2}{1-D}\notag\\
&+\frac{D}{1-D}\frac{1}{K} \sum_{i=1}^K\mathbb{E}\left[\norm{\nabla F(\overline{x}_k)}^2\right].
\end{align}
Therefore,
\begin{align}
    \sum_{i=1}^K\mathbb{E}\left[\norm{\nabla F(\overline{x}_k)}^2\right]\leq &\left(\frac{2(F(\overline{x}_{1})-F^*)}{\eta K}+\frac{2M}{\eta}\right)\frac{1-D}{1-2D}+\left(\frac{2\eta^2L^2\rho(m\sigma^2+\lambda^2\delta^2)}{m(1-\rho)}+\frac{6\eta^2L^2\zeta^2\rho}{(1-\sqrt{\rho})^2}\right)\frac{1}{1-2D}\notag\\
    \leq&\left(\frac{2(F(\overline{x}_{1})-F^*)}{\eta K}+\frac{2M}{\eta}\right)\frac{1}{1-2D}+\frac{2\eta^2L^2\rho}{1-\sqrt{\rho}}\left(\frac{m\sigma^2+\lambda^2\delta^2}{m(1+\sqrt{\rho})}+\frac{3\zeta^2}{1-\sqrt{\rho}}\right)\frac{1}{1-2D}
\end{align}
Recall that $\eta L\leq(1-\sqrt{\rho})/4\sqrt{\rho}$, we could know that $\frac{1}{1-2D}\leq 4$. Therefore the bound could be simplified as
\begin{align}
 \sum_{i=1}^K\mathbb{E}\left[\norm{\nabla F(\overline{x}_k)}^2\right]\leq\frac{8(F(\overline{x}_{1})-F^*)}{\eta K}+\frac{8M}{\eta}+\frac{8\eta^2L^2\rho}{1-\sqrt{\rho}}\left(\frac{m\sigma^2+\lambda^2\delta^2}{m(1+\sqrt{\rho})}+\frac{3\zeta^2}{1-\sqrt{\rho}}\right),
\end{align}
where $M=\frac{\eta^2L\sigma^2}{2m}+\lambda\eta\beta\delta+\lambda\eta^2L\beta \delta+\frac{\lambda^2\eta^2L\delta^2}{2}$.
When $\eta=\lambda=\sqrt{\frac{m}{K}}$,
\begin{align}
    \sum_{i=1}^K\mathbb{E}\left[\norm{\nabla F(\overline{x}_k)}^2\right]\leq& \frac{8(F(\overline{x}_{1})-F^*)}{\sqrt{mK}}+\frac{4 L\sigma^2}{\sqrt{mk}}+8\beta\delta\sqrt{\frac{m}{K}}+8\lambda L\beta \delta\sqrt{\frac{m}{K}}+4\lambda^2 L\delta^2\sqrt{\frac{m}{K}}\notag\\
    &+\frac{8\sqrt{m} L^2\rho}{(1-\sqrt{\rho})\sqrt{K}}\left(\frac{\sigma^2}{1+\sqrt{\rho}}+\frac{\delta^2}{K(1+\sqrt{\rho})}+\frac{3\zeta^2}{1-\sqrt{\rho}}\right)\notag\\
    =&\mathcal{O}(\frac{1}{\sqrt{mK}})+\mathcal{O}(\sqrt{\frac{m}{K}})+ +\mathcal{O}(\sqrt{\frac{m}{K^3}})
\end{align}
